# Supplementary material for: Conditional inference for high-dimensional multi-omics survival data
Source: arXiv:2504.21324 source file (2025-10-06)
Supplement: Supplementary file 1 [file suppwithauthors.tex]

% Options for packages loaded elsewhere
\PassOptionsToPackage{unicode}{hyperref}
\PassOptionsToPackage{hyphens}{url}
\PassOptionsToPackage{dvipsnames,svgnames,x11names}{xcolor}
\documentclass[
  12pt]{article}

\usepackage{amsmath,amssymb}
\usepackage{iftex}
\ifPDFTeX
  \usepackage[T1]{fontenc}
  \usepackage[utf8]{inputenc}
  \usepackage{textcomp} % provide euro and other symbols
\else % if luatex or xetex
  \usepackage{unicode-math}
  \defaultfontfeatures{Scale=MatchLowercase}
  \defaultfontfeatures[\rmfamily]{Ligatures=TeX,Scale=1}
\fi
\usepackage{lmodern}
\ifPDFTeX\else  
    % xetex/luatex font selection
\fi
% Use upquote if available, for straight quotes in verbatim environments
\IfFileExists{upquote.sty}{\usepackage{upquote}}{}
\IfFileExists{microtype.sty}{% use microtype if available
  \usepackage[]{microtype}
  \UseMicrotypeSet[protrusion]{basicmath} % disable protrusion for tt fonts
}{}
\makeatletter
\@ifundefined{KOMAClassName}{% if non-KOMA class
  \IfFileExists{parskip.sty}{%
    \usepackage{parskip}
  }{% else
    \setlength{\parindent}{0pt}
    \setlength{\parskip}{6pt plus 2pt minus 1pt}}
}{% if KOMA class
  \KOMAoptions{parskip=half}}
\makeatother
\usepackage{xcolor}
\setlength{\emergencystretch}{3em} % prevent overfull lines
\setcounter{secnumdepth}{5}
% Make \paragraph and \subparagraph free-standing
\makeatletter
\ifx\paragraph\undefined\else
  \let\oldparagraph\paragraph
  \renewcommand{\paragraph}{
    \@ifstar
      \xxxParagraphStar
      \xxxParagraphNoStar
  }
  \newcommand{\xxxParagraphStar}[1]{\oldparagraph*{#1}\mbox{}}
  \newcommand{\xxxParagraphNoStar}[1]{\oldparagraph{#1}\mbox{}}
\fi
\ifx\subparagraph\undefined\else
  \let\oldsubparagraph\subparagraph
  \renewcommand{\subparagraph}{
    \@ifstar
      \xxxSubParagraphStar
      \xxxSubParagraphNoStar
  }
  \newcommand{\xxxSubParagraphStar}[1]{\oldsubparagraph*{#1}\mbox{}}
  \newcommand{\xxxSubParagraphNoStar}[1]{\oldsubparagraph{#1}\mbox{}}
\fi
\makeatother

\usepackage{longtable,booktabs,array}
\usepackage{calc} % for calculating minipage widths
% Correct order of tables after \paragraph or \subparagraph
\usepackage{etoolbox}
\makeatletter
\patchcmd\longtable{\par}{\if@noskipsec\mbox{}\fi\par}{}{}
\makeatother
% Allow footnotes in longtable head/foot
\IfFileExists{footnotehyper.sty}{\usepackage{footnotehyper}}{\usepackage{footnote}}
\makesavenoteenv{longtable}
\usepackage{graphicx}
\makeatletter
\def\maxwidth{\ifdim\Gin@nat@width>\linewidth\linewidth\else\Gin@nat@width\fi}
\def\maxheight{\ifdim\Gin@nat@height>\textheight\textheight\else\Gin@nat@height\fi}
\makeatother
% Scale images if necessary, so that they will not overflow the page
% margins by default, and it is still possible to overwrite the defaults
% using explicit options in \includegraphics[width, height, ...]{}
\setkeys{Gin}{width=\maxwidth,height=\maxheight,keepaspectratio}
% Set default figure placement to htbp
\makeatletter
\def\fps@figure{htbp}
\makeatother

\addtolength{\oddsidemargin}{-.5in}%
\addtolength{\evensidemargin}{-.1in}%
\addtolength{\textwidth}{1in}%
\addtolength{\textheight}{1.7in}%
\addtolength{\topmargin}{-1in}
\makeatletter
\@ifpackageloaded{caption}{}{\usepackage{caption}}
\AtBeginDocument{%
\ifdefined\contentsname
  \renewcommand*\contentsname{Table of contents}
\else
  \newcommand\contentsname{Table of contents}
\fi
\ifdefined\listfigurename
  \renewcommand*\listfigurename{List of Figures}
\else
  \newcommand\listfigurename{List of Figures}
\fi
\ifdefined\listtablename
  \renewcommand*\listtablename{List of Tables}
\else
  \newcommand\listtablename{List of Tables}
\fi
\ifdefined\figurename
  \renewcommand*\figurename{Figure}
\else
  \newcommand\figurename{Figure}
\fi
\ifdefined\tablename
  \renewcommand*\tablename{Table}
\else
  \newcommand\tablename{Table}
\fi
}
\@ifpackageloaded{float}{}{\usepackage{float}}
\floatstyle{ruled}
\@ifundefined{c@chapter}{\newfloat{codelisting}{h}{lop}}{\newfloat{codelisting}{h}{lop}[chapter]}
\floatname{codelisting}{Listing}

\makeatother
\makeatletter
\makeatother
\makeatletter
\@ifpackageloaded{caption}{}{\usepackage{caption}}
\@ifpackageloaded{subcaption}{}{\usepackage{subcaption}}
\makeatother

\ifLuaTeX
  \usepackage{selnolig}  % disable illegal ligatures
\fi
\usepackage[]{natbib}
\bibliographystyle{agsm}
\usepackage{bookmark}

\IfFileExists{xurl.sty}{\usepackage{xurl}}{} % add URL line breaks if available
\urlstyle{same} % disable monospaced font for URLs
\hypersetup{
  pdftitle={Title},
  pdfauthor={Author 1; Author 2},
  pdfkeywords={3 to 6 keywords, that do not appear in the title},
  colorlinks=true,
  linkcolor={blue},
  filecolor={Maroon},
  citecolor={Blue},
  urlcolor={Blue},
  pdfcreator={LaTeX via pandoc}}

\newcommand{\bbR}{\mathbb{R}}
\newcommand{\bbE}{\mathbb{E}}

\newcommand{\bI}{\mathbf{I}}

\newcommand{\bB}{\mathbf{B}}

\newcommand{\bZ}{\mathbf{Z}}

\newcommand{\bW}{\mathbf{W}}

\newcommand{\vf}{\mathbf{f}}

\newcommand{\bx}{\mathbf{x}}
\newcommand{\by}{\mathbf{y}}
\newcommand{\bz}{\mathbf{z}}

\newcommand{\bs}{\mathbf{s}}
\newcommand{\bS}{\mathbf{S}}
\newcommand{\bT}{\mathbf{T}}
\newcommand{\bu}{\mathbf{u}}

\newcommand{\bH}{\mathbf{H}}

\newcommand{\bw}{\mathbf{w}}

\newcommand{\bvarepsilon}{\boldsymbol{\varepsilon}}

\newcommand{\bbeta}{\boldsymbol{\beta}}

\newcommand{\btheta}{\boldsymbol{\theta}}

\newcommand{\bphi}{\boldsymbol{\phi}}
\newcommand{\bPhi}{\boldsymbol{\Phi}}

\newcommand{\bSigma}{\boldsymbol{\Sigma}}

\newcommand{\bgamma}{\boldsymbol{\gamma}}

\newcommand{\bxi}{\boldsymbol{\xi}}
\newcommand{\bDelta}{\boldsymbol{\Delta}}

%------------------------------------------------------------
% Theorem like environments
%

%\newtheorem{algorithm}{Algorithm}
%\newtheorem{axiom}{Axiom}

\newtheorem{lemma}{Lemma}

\usepackage{xr}
\externaldocument{main}

%set the key \texttt{anon} to ``0'' to hide the authors and acknowledgements,
%  producing the required anonymized version. 
%Set the key \texttt{anon} to ``1'' to produce the manuscript with author details and
% acknowledgments. 

\begin{document}

\def\spacingset#1{\renewcommand{\baselinestretch}%
{#1}\small\normalsize} \spacingset{1}

%%%%%%%%%%%%%%%%%%%%%%%%%%%%%%%%%%%%%%%%%%%%%%%%%%%%%%%%%%%%%%%%%%%%%%%%%%%%%%

\spacingset{1.8} % DON'T change the spacing!

\renewcommand{\thesection}{S\arabic{section}}
\setcounter{section}{0}

\begin{center}
{\Large\bf \textsf{Supplementary Material to ``Conditional inference for high-dimensional multi-omics survival data"}}
\end{center}

\vspace*{0.1in}

\begin{center}
{Heyuan Zhang$^{1,2}$, Meiling Hao$^{3}$, Lianqiang Qu$^{4}$, and Liuquan Sun$^{1,2}$}\\
 \small{\sl$^1$SKLMS, Academy of Mathematics and Systems Science, Chinese Academy of Sciences, China}\\
 \small{\sl$^2$School of Mathematical Sciences, University of Chinese Academy of Sciences, China\\}
 \small{\sl$^3$School of Statistics, University of International Business and Economics, China\\}
 \small{\sl$^4$School of Mathematics and Statistics, Central China Normal University,  China}
\end{center}

In the Supplementary Materials, we provide proofs of the main theorems along with related technical lemmas.
For simplicity, denote \( \bxi_{i,m}^* = \vf_{i,m} - {\bW^*}^\top \bx_{i,-m} \).

\setcounter{equation}{0}
\renewcommand{\theequation}{S.\arabic{equation}}

\section{Proof of Theorem~\ref{theorem1}} 
	
To prove Theorem~\ref{theorem1}, it suffices to establish the following two results:
	\begin{align}
		\sqrt{n}\bSigma_{\bgamma_m|\bbeta_{-m}}^{*-1/2}\bS(\hat{\bbeta}_{-m},\mathbf{0};\hat{\bxi}_m)&\stackrel{d}{\longrightarrow}N(\mathbf 0,\bI_{K_m}), \label{S1} \\
		\mbox{and}\,\,\hat\bSigma_{\bgamma_m|\bbeta_{-m}}&\stackrel{p}{\longrightarrow}\bSigma^*_{\bgamma_m|\bbeta_{-m}}. \label{S2} 
	\end{align}
    Then by (\ref{S1}) and (\ref{S2}), Theorem~\ref{theorem1} follows directly from Slutsky's theorem.
    
 For convenience, we first define
    $$
    \begin{aligned}
        \bPhi_{\bxi_m^*} (t)&=\frac{\sum_{j=1}^nY_j(t)\exp(\bx_{j,-m}^\top\bbeta_{-m}^*){\bxi}_{j,m}^*}{\sum_{j=1}^nY_j(t)\exp(\bx_{j,-m}^\top\bbeta_{-m}^*)},\\
        \bphi_{\bxi_m^*} (t)&=\frac{\bbE [Y_1(t)\exp(\bx_{1,-m}^\top\bbeta_{-m}^*){\bxi}_{1,m}^*]}{\bbE [Y_1(t)\exp(\bx_{1,-m}^\top\bbeta_{-m}^*)]}.
    \end{aligned}
    $$
    The functional central limit theorem \citep{pollard1990empirical} implies  $\sup_{t\in [0,\tau]} \left\|\bPhi_{\bxi_m^*} (t)-\bphi_{\bxi_m^*} (t)\right\|_\infty=O_p(n^{-1/2})$. 
    
  \noindent{Step I:} In the following , we first prove  (\ref{S1}). Observe that
    $$
    \begin{aligned}
        \bS({\bbeta}_{-m}^*,\mathbf{0};{\bxi}_m^*)=-\frac{1}{n}\sum_{i=1}^n\int_0^\tau\bigg[{\bxi}_{i,m}^*- \bPhi_{\bxi_m^*} (t)\bigg]dM_i(t;\bbeta_{-m}^*),
    \end{aligned}
    $$
    where $M_i(t;\bbeta^*_{-m})=N_i(t)-\int_0^t Y_i(u)\lambda_0(u)\exp(\bx_{i,-m}^\top\bbeta^*_{-m})du$.
    Then it is sufficient to show $\bS(\hat{\bbeta}_{-m},\mathbf{0};\hat{\bxi}_m)-\bS({\bbeta}_{-m}^*,\mathbf{0};{\bxi}_m^*)=o_p(n^{-1/2})$ since by the central limit theorem and the Slutsky's theorem,
$$\sqrt{n}\bSigma_{\bgamma_m|\bbeta_{-m}}^{*-1/2}\bS({\bbeta}_{-m}^*,\mathbf{0};{\bxi}_m^*)\stackrel{d}{\longrightarrow}N(\mathbf 0,\bI_{K_m}).$$ 
Note that
	\begin{align*}
	&\bS(\hat{\bbeta}_{-m},\mathbf{0};\hat{\bxi}_m)-\bS({\bbeta}_{-m}^*,\mathbf{0};{\bxi}_m^*)\\
    =&\big[\bS(\hat{\bbeta}_{-m},\mathbf{0};\hat{\bxi}_m)-\bS({\bbeta}_{-m}^*,\mathbf{0};\hat{\bxi}_m)\big]+\big[\bS({\bbeta}_{-m}^*,\mathbf{0};\hat{\bxi}_m)-\bS({\bbeta}_{-m}^*,\mathbf{0};{\bxi}_m^*)\big]\\
    =&I_1+I_2,
	\end{align*}
	where
	$$
	\bS({\bbeta}_{-m}^*,\mathbf{0};\hat{\bxi}_m)=-\frac{1}{n}\sum_{i=1}^n\int_0^\tau\bigg[\hat{\bxi}_{i,m}-\frac{\sum_{j=1}^nY_j(t)\exp(\bx_{j,-m}^\top\bbeta_{-m}^*)\hat{\bxi}_{j,m}}{\sum_{j=1}^nY_j(t)\exp(\bx_{j,-m}^\top\bbeta_{-m}^*)}\bigg]dM_i(t;\bbeta_{-m}^*).
	$$

For $I_1$, let $\gamma_{m_k}$ be the $k$-th element of $\bgamma_m$ and $\hat\bw_k$ be the $k$-th column of $\hat\bW$.
By applying the Taylor expansion, for the $k$-th element of $I_1$, denoted as $I_{1,k}$, we have 
$$
	\begin{aligned}
	\left|I_{1,k}\right|&=\left|\frac1n\sum_{i=1}^n\int_0^\tau\bigg[\frac{\sum_{j=1}^nY_j(t)\exp(\bx_{j,-m}^\top\bbeta_{-m}^*)\hat{\xi}_{j,m_k}}{\sum_{j=1}^nY_j(t)\exp(\bx_{j,-m}^\top\bbeta_{-m}^*)}-\frac{\sum_{j=1}^nY_j(t)\exp(\bx_{j,-m}^\top\hat\bbeta_{-m})\hat{\xi}_{j,m_k}}{\sum_{j=1}^nY_j(t)\exp(\bx_{j,-m}^\top\hat\bbeta_{-m})}\bigg]dN_i(t)\right|\\
	&=\left| \left\{\nabla^2_{\gamma_{m_k},\bbeta_{-m}} l(\hat\bbeta_{-m},0;\hat{\vf}_m)-\hat\bw_k^\top\nabla^2_{\bbeta_{-m},\bbeta_{-m}} l(\hat\bbeta_{-m},0;\hat{\vf}_m)\right\}(\bbeta_{-m}^*-\hat\bbeta_{-m})\left\{1+o_p(1)\right\}\right| \\
	&\leq\left\| \nabla^2_{\gamma_{m_k},\bbeta_{-m}}l(\hat\bbeta_{-m},0;\hat{\vf}_m)-\hat\bw_k^\top\nabla^2_{\bbeta_{-m},\bbeta_{-m}} l(\hat\bbeta_{-m},0;\hat{\vf}_m) \right\|_\infty\left\|\bbeta_{-m}^*-\hat\bbeta_{-m}\right\|_1\left\{1+o_p(1)\right\}   \\
        &\le\lambda_2 \left\|\bbeta_{-m}^*-\hat\bbeta_{-m}\right\|_1\left\{1+o_p(1)\right\}.
	\end{aligned}
    $$
    The last inequality follows from (\ref{w_hat}) in the main text.
    It follows from Lemma \ref{lemm2} that $\|\bbeta_{-m}^*-\hat\bbeta_{-m}\|_1=O_p(s_{-m}^*\lambda_1) $, where $s_{-m}^*=\left|\text{supp}(\bbeta_{-m}^*)\right| $. Note that 
    $$
    n^{1/2}s^*_{-m}C_{n,p_m,p-p_m}C_{n,p_m,p-p_m}^\prime=o(1).
    $$ 
    Thus, we have $\left|I_{1,k}\right|=o_p(n^{-1/2})$.
    
    For $I_2$, we have
    $$
    \begin{aligned}
    	-I_2=&\frac{1}{n}\sum_{i=1}^n\int_0^\tau\bigg[(\hat{\bxi}_{i,m}-\bxi_{i,m}^*)-\frac{\sum_{j=1}^nY_j(t)\exp(\bx_{j,-m}^\top\bbeta_{-m}^*)(\hat{\bxi}_{j,m}-\bxi_{j,m}^*)}{\sum_{j=1}^nY_j(t)\exp(\bx_{j,-m}^\top\bbeta_{-m}^*)}\bigg]dM_i(t;\bbeta_{-m}^*) \\
    	=&\frac{1}{n}\sum_{i=1}^n\int_0^\tau\bigg[(\hat{\vf}_{i,m}-\vf_{i,m})-\frac{\sum_{j=1}^nY_j(t)\exp(\bx_{j,-m}^\top\bbeta_{-m}^*)(\hat{\vf}_{j,m}-\vf_{j,m})}{\sum_{j=1}^nY_j(t)\exp(\bx_{j,-m}^\top\bbeta_{-m}^*)}\bigg]dM_i(t;\bbeta_{-m}^*)\\
    	&-\frac{1}{n}\sum_{i=1}^n\int_0^\tau(\hat{\bW}-\bW^*)^\top\bigg[\bx_{i,-m}-\frac{\sum_{j=1}^nY_j(t)\exp(\bx_{j,-m}^\top\bbeta_{-m}^*)\bx_{j,-m}}{\sum_{j=1}^nY_j(t)\exp(\bx_{j,-m}^\top\bbeta_{-m}^*)}\bigg]dM_i(t;\bbeta_{-m}^*) \\
    	=&I_2^{(1)}-I_2^{(2)}.
    \end{aligned}
    $$
    When 
    $$
    \max_{i\in[n]}\|\hat{\vf}_{i,m}-\vf_{i,m}\|_\infty\le C\left[\sqrt{\frac{\log(n)}{p_m}}+\sqrt{\frac{\log (p_m)\log (n)}{n}}\right]
    $$
    for some positive constant $C>0$, let $\hat{\vf}_{i,m}-\vf_{i,m}=\bvarepsilon_iC\left[\sqrt{\log (n)/{p_m}}+\sqrt{\log (p_m)\log (n)/{n}}\right]$, where $\mathbb E\bvarepsilon_i=0$ and $\left\|\bvarepsilon_i\right\|_\infty\le1$ for $i\in[n]$. Let $\mathbb B(\bx,r)=\left\{\by\in\mathbb R^{K_m}:\left\|\by-\bx\right\|_\infty< r\right\}$. Then $\bar{\mathbb B}(\boldsymbol 0,1)$ is totally bounded in $\mathbb R^{K_m}$ and thus has finite $\varepsilon$-nets, which means that for any $\varepsilon>0$, there exist $\bs_1,\dots,\bs_q\in \bar{\mathbb B}(\boldsymbol 0,1)$ such that $\bar{\mathbb B}(\boldsymbol 0,1)\subset\bigcup_{t=1}^q{\mathbb B}(\bs_t,\varepsilon)$. For any independent random variables $\bvarepsilon_{1,t},\dots,\bvarepsilon_{n,t}\in {\mathbb B}(\bs_t,\varepsilon)\bigcap\bar{\mathbb B}(\boldsymbol 0,1)$ with zero means, by the Bernstein inequality, we have 
    $$
    \begin{aligned}
        &\mathbb P\left[\left\|\frac{1}{n}\sum_{i=1}^n\int_0^\tau\left\{\bvarepsilon_{i,t}-\frac{\sum_{j=1}^nY_j(t)\exp(\bx_{j,-m}^\top\bbeta_{-m}^*)\bvarepsilon_{j,t}}{\sum_{j=1}^nY_j(t)\exp(\bx_{j,-m}^\top\bbeta_{-m}^*)}\right\}dM_i(t;\bbeta_{-m}^*)\right\|_\infty
        \ge \frac{t}{\sqrt{n}} \right] \\
        &\le 2K_m\exp(-\frac{3t^2}{6+2t}).
    \end{aligned}
    $$
    Then by the union bound, we have
    $$
    \begin{aligned}
        &\mathbb P\left[\left\|\frac{1}{n}\sum_{i=1}^n\int_0^\tau\left\{\bvarepsilon_{i}-\frac{\sum_{j=1}^nY_j(t)\exp(\bx_{j,-m}^\top\bbeta_{-m}^*)\bvarepsilon_{j}}{\sum_{j=1}^nY_j(t)\exp(\bx_{j,-m}^\top\bbeta_{-m}^*)}\right\}dM_i(t;\bbeta_{-m}^*)\right\|_\infty
        \ge \frac{t}{\sqrt{n}} \right] \\
        &\le 2qK_m\exp(-\frac{3t^2}{6+2t}).
    \end{aligned}
    $$
    Since $K_m$ is fixed, together with Lemma~\ref{lemm1} below, we have 
    $$
    \left\|I_2^{(1)}\right\|_\infty=O_p\left[n^{-1/2}\left\{\sqrt{\log (n)/{p_m}}+\sqrt{\log (p_m)\log (n)/{n}}\right\}\right]=o_p(n^{-1/2}).
    $$
    For the $k$-th element of $I_2^{(2)}$, denoted as $I_{2,k}^{(2)}$, by Lemma~\ref{lemm2} and the fact that 
    $$
    \sup_{t\in (0,\tau)} \left\|\bPhi_{\bx_{-m}} (t)-\bphi_{\bx_{-m}} (t)\right\|_\infty=O_p\left[\sqrt{\log (p-p_m)/n}\right],
    $$
    we have
    $$
    \begin{aligned}
        \left|I_{2,k}^{(2)}\right|&=\left|\frac{1}{n}\sum_{i=1}^n\int_0^\tau(\hat{\bw}_k-\bw_k^*)^\top\bigg[\bx_{i,-m}-\frac{\sum_{j=1}^nY_j(t)\exp(\bx_{j,-m}^\top\bbeta_{-m}^*)\bx_{j,-m}}{\sum_{j=1}^nY_j(t)\exp(\bx_{j,-m}^\top\bbeta_{-m}^*)}\bigg]dM_i(t;\bbeta_{-m}^*)\right| \\
        &\le\left\|\hat{\bw}_k-\bw_k^*\right\|_1\left\| \frac{1}{n}\sum_{i=1}^n\int_0^\tau\bigg[\bx_{i,-m}-\frac{\sum_{j=1}^nY_j(t)\exp(\bx_{j,-m}^\top\bbeta_{-m}^*)\bx_{j,-m}}{\sum_{j=1}^nY_j(t)\exp(\bx_{j,-m}^\top\bbeta_{-m}^*)}\bigg]dM_i(t;\bbeta_{-m}^*)\right\|_\infty \\
        &=O_p(s_k^*\lambda_2) O_p\left[\sqrt{\log (p-p_m)/n}\right] \\
        &=o_p(n^{-1 / 2}),
    \end{aligned}
    $$
    where $s_k^*=\left|\text{supp}(\bw_k^*)\right| $. This completes the proof for (\ref{S1}).

   \noindent{Step II:}  Now, we  prove (\ref{S2}). Since $K_m$ is fixed, all matrix norms are equivalent. First, we will show 
    $$
    \left\|\hat\bSigma_{\bgamma_m|\bbeta_{-m}}-\bSigma^*_{\bgamma_m|\bbeta_{-m}}\right\|_\infty=o_p(1).
    $$
    Recall 
    $$
    \begin{aligned}
        \bSigma^*_{\bgamma_m|\bbeta_{-m}}&= \bSigma^*_{\bgamma_m,\bgamma_m}-\bW^{*\top}\bSigma^*_{\bbeta_{-m},\bgamma_m}, \\
        \hat\bSigma_{\bgamma_m|\bbeta_{-m}} &= \nabla^2_{\bgamma_m,\bgamma_m}{l}(\hat\bbeta_{-m},\hat\bgamma_{m};\hat{\vf}_m)-\hat\bW^\top \nabla^2_{\bbeta_{-m},\bgamma_m} {l}(\hat\bbeta_{-m},\hat\bgamma_{m};\hat{\vf}_m).  
    \end{aligned}
    $$
    By Lemma B.2 of \cite{fan2022}, we have 
    \begin{align} \label{S3}
    \left\|\nabla^2_{\bbeta_{-m}\bgamma_m}{l}(\hat\bbeta_{-m},\hat\bgamma_{m};\hat{\vf}_m)-\bSigma^*_{\bbeta_{-m}\bgamma_m}\right\|_\infty=O_p\left\{\sqrt{s^*_{-m}}\left(\sqrt{\frac{\log (p-p_m)}{n}}+\frac{1}{\sqrt{p_m}}\right)\right\}.
    \end{align}
    For the $k$-th row, we have
    $$
    \begin{aligned}
        &\left\|\hat\bw_k^\top \nabla^2_{\bbeta_{-m},\bgamma_m} {l}(\hat\bbeta_{-m},\hat\bgamma_{m};\hat{\vf}_m)-\bw_k^{*\top}\bSigma^*_{\bbeta_{-m},\bgamma_m}\right\|_\infty \\
        \le&
        \left\|\left(\hat\bw_k-\bw_k^*\right)^\top \nabla^2_{\bbeta_{-m},\bgamma_m} {l}(\hat\bbeta_{-m},\hat\bgamma_{m};\hat{\vf}_m)\right\|_\infty \\
        +& 
        \left\|\bw_k^{*\top}\left\{\nabla^2_{\bbeta_{-m},\bgamma_m} {l}(\hat\bbeta_{-m},\hat\bgamma_{m};\hat{\vf}_m)-\bSigma^*_{\bbeta_{-m},\bgamma_m}\right\}\right\|_\infty.
    \end{aligned}
    $$
    For the first term, let $\gamma_{m,h}$ be the $h$-th element of $\bgamma_m$. Then we have
    $$
    \begin{aligned}
         &\left\|\left(\hat\bw_k-\bw_k^*\right)^\top \nabla^2_{\bbeta_{-m},\bgamma_m} {l}(\hat\bbeta_{-m},\hat\bgamma_{m};\hat{\vf}_m)\right\|_\infty\\
         =&\max_{h\in[K_m]}\left|\left(\hat\bw_k-\bw_k^*\right)^\top \nabla^2_{\bbeta_{-m},\gamma_{m,h}} {l}(\hat\bbeta_{-m},\hat\bgamma_{m};\hat{\vf}_m)\right|\\
         \le&\left\|\hat{\bw}_k-\bw_k^* \right\|_1 \cdot \max_{h\in[K_m]}\left\| \nabla^2_{\bbeta_{-m},\gamma_{m,h}} {l}(\hat\bbeta_{-m},\hat\bgamma_{m};\hat{\vf}_m) \right\|_{\infty} \\
         \le&\left\|\hat{\bw}_k-\bw_k^* \right\|_1 \cdot \max_{h\in[K_m]}\left\{\left\| \nabla^2_{\bbeta_{-m},\gamma_{m,h}} {l}(\hat\bbeta_{-m},\hat\bgamma_{m};\hat{\vf}_m)-\bSigma^*_{\bbeta_{-m},\gamma_{m,h}}\right\|_{\infty}+\left\|\bSigma^*_{\bbeta_{-m},\gamma_{m,h}}\right\|_\infty\right\} \\
         =&O_p (s_k^*\lambda_2) O_p(1)  \\
         =&o_p(1),
    \end{aligned}
    $$
    where the second last equality follows from Lemma~\ref{lemm2}, (\ref{S3}) and the fact that $\|\bSigma^*_{\bbeta_{-m},\gamma_{m,h}}\|_\infty=O(1)$ . For the second term,
    $$
    \begin{aligned}
        &\left\|\bw_k^{*\top}\left\{\nabla^2_{\bbeta_{-m},\bgamma_m} {l}(\hat\bbeta_{-m},\hat\bgamma_{m};\hat{\vf}_m)-\bSigma^*_{\bbeta_{-m},\bgamma_m}\right\}\right\|_\infty \\
        =&\max_{h\in[K_m]}\left|\bw_k^{*\top}\left\{\nabla^2_{\bbeta_{-m},\gamma_{m,h}} {l}(\hat\bbeta_{-m},\hat\bgamma_{m};\hat{\vf}_m)-\bSigma^*_{\bbeta_{-m},\gamma_{m,h}}\right\}\right| \\
        \le&\left\|\bw_k^* \right\|_1\cdot\max_{h\in[K_m]}\left\{\left\|\nabla^2_{\bbeta_{-m},\gamma_{m,h}} {l}(\hat\bbeta_{-m},\hat\bgamma_{m};\hat{\vf}_m)-\nabla^2_{\bbeta_{-m},\bbeta_{-m}} {l}(\hat\bbeta_{-m},\hat\bgamma_{m};\hat{\vf}_m)\bw_h^*\right\|_\infty\right. \\
        &+\left.\left\|\nabla^2_{\bbeta_{-m},\bbeta_{-m}} {l}(\hat\bbeta_{-m},\hat\bgamma_{m};\hat{\vf}_m)\bw_h^*-\bSigma^*_{\bbeta_{-m},\bbeta_{-m}}\bw_h^* \right\|_\infty\right\} \\
        =&O_p (s_k^*C^\prime_{n,p_m,p-p_m})   \\
        =&o_p(1),
    \end{aligned}
    $$
    where the the second last equality follows from Lemma~\ref{lemma3} below and the central limit theorem. This completes the proof for (\ref{S2}).

    \section{Proof of Theorem~\ref{theorem2}}
    
Letting $A_n=\|\bT_n\|_2^2,\bT_n^*=\sqrt{n} \bSigma_{\bgamma_m \mid \bbeta_{-m}}^{{*-1 / 2}}\left\{\bS\left(\bbeta^*, \bgamma_m^*;\bxi^*\right)-\bSigma^*_{\bgamma_m \mid \bbeta_{-m}} \bgamma_m^*\right\}$, and $A_n^*=\|\bT_n^*\|_2^2$. By arguments similar to those in Lemmas 9–11 of \cite{li2021integrative},  we have  $\bT_n^*=\bT_n+o_p(1)$. Together with the continuous mapping theorem, we obtain that $A_n=A_n^*+o_p(1)$.

    Next, we derive the asymptotic distribution of $A_n^*$. By definition,
    $$
    \begin{aligned}
         \bT_n^*=&\sqrt{n} \bSigma_{\bgamma_m \mid \bbeta_{-m}}^{{*-1 / 2}}\left\{\bS\left(\bbeta^*, \bgamma_m^*;\bxi^*\right)-\bSigma^*_{\bgamma_m \mid \bbeta_{-m}} \bgamma_m^*\right\} \\ 
         =&-\frac{1}{\sqrt{n}} \bSigma_{\bgamma_m \mid \bbeta_{-m}}^{{*-1 / 2}}\sum_{i=1}^n\int_0^\tau\bigg[\bxi_{i,m}^*-\frac{\sum_{j=1}^nY_j(t)\exp(\vf_{j,m}^\top\bgamma_m^*+\bz_j^\top\bbeta^*)\bxi_{j,m}^*}{\sum_{j=1}^nY_j(t)\exp(\vf_{j,m}^\top\bgamma_m^*+\bz_j^\top\bbeta^*)}\bigg] dM_i(t;\bgamma_m^*,\bbeta^*) \\
         &-\sqrt{n}\bSigma_{\bgamma_m \mid \bbeta_{-m}}^{*1/2} \bgamma_m^* \\
         =&\sum_{i=1}^n\boldsymbol{\eta}_i-\sqrt{n}\bSigma_{\bgamma_m \mid \bbeta_{-m}}^{*1/2} \bgamma_m^*+o_p(1),
    \end{aligned}
    $$
    where
    $$
    \boldsymbol{\eta}_i=-\frac{1}{\sqrt{n}} \bSigma_{\bgamma_m \mid \bbeta_{-m}}^{{*-1 / 2}}\int_0^\tau\bigg[\bxi_{i,m}^*-\frac{\bbE \{Y_1(t)\exp(\vf_{1,m}^\top\bgamma_m^*+\bz_1^\top\bbeta^*)\bxi_{1,m}^*\}}{\bbE \{Y_1(t)\exp(\vf_{1,m}^\top\bgamma_m^*+\bz_1^\top\bbeta^*)\}}\bigg] dM_i(t;\bgamma_m^*,\bbeta^*).
    $$
    Direct calculations show that $\bbE(\boldsymbol{\eta}_i)=0$, and $\sum_{i=1}^n\operatorname{var}(\boldsymbol{\eta}_i)=\bI_{K_m}$. By Lemma 4 of \cite{li2021integrative}, we have
    $$
    \sup _{C}\left|\mathbb{P}\left(\sum_{i=1}^n \boldsymbol{\eta}_i \in C\right)-\mathbb{P}(\bZ \in C)\right| \rightarrow 0,
    $$
    where the supremum is taken over all convex sets $C\in \bbR^{K_m}$ and $\bZ\sim N(0,\bI_{K_m})$. Let $C=\{\bz\in\bbR^{K_m}:\|\bz-\sqrt{n}\bSigma_{\bgamma_m \mid \bbeta_{-m}}^{*1/2} \bgamma_m^*\|_2^2\le x\}$. Then
    $$
    \sup _x\left|\mathbb{P}\left(A_n^* \leq x\right)-\mathbb{P}\left\{\chi^2\left(K_m, d_n\right) \leq x\right\}\right|=\sup _x\left|\mathbb{P}\Big(\sum_{i=1}^n \boldsymbol{\eta}_i \in C\Big)-\mathbb{P}(\bZ \in C)\right| \rightarrow 0,
    $$
    where $d_n=n\bgamma_m^*\bSigma^*_{\bgamma_m|\bbeta_{-m}}\bgamma^*_m$. Since $A_n=A_n^*+o_p(1)$, for any $x$ and $\varepsilon>0$, we have 
    $$
    \begin{aligned}
        &\mathbb{P}\left\{\chi^2\left(K_m, d_n\right)\le x-\varepsilon\right\}+o(1)\le \mathbb{P}(A_n^*\le x-\varepsilon)+o(1) \le\mathbb{P}(A_n\le x) \\
        &\le \mathbb{P}(A_n^*\le x+\varepsilon)+o(1) \le \mathbb{P}\left\{\chi^2\left(K_m, d_n\right)\le x+\varepsilon\right\}+o(1).
    \end{aligned}
    $$
    On the other hand, it follows from Lemma 5 of \cite{li2021integrative} that 
    $$
    \lim_{\varepsilon\to 0}\limsup_n|\mathbb{P}\left\{\chi^2\left(K_m, d_n\right)\le x+\varepsilon\right\}-\mathbb{P}\left\{\chi^2\left(K_m, d_n\right)\le x-\varepsilon\right\}|\to 0.
    $$
    Thus, we have
    $$
    \sup _x\left|\mathbb{P}\left(A_n \leq x\right)-\mathbb{P}\left\{\chi^2\left(K_m, d_n\right) \leq x\right\}\right| \rightarrow 0.
    $$

    \vspace{0.1in}

    \section{Proof of Lemma~\ref{lemm2}}
    
  We first calculate the estimation error of $\hat{\bbeta}_{-m}$ in the presence of factor estimation. By Theorem 3.1 of \cite{lasso2013}, on the event 
  $$
  \|\nabla l(\bbeta^*_{-m},\bgamma^*_m;\hat{\vf}_m)\|_\infty\le\lambda_1(\xi-1)/(\xi+1),
  $$ 
  we have $\|\hat\bbeta_{-m}-\bbeta_{-m}^*\|_1=O_p(s_{-m}^*\lambda_1)$. Thus, to bound $\|\hat\bbeta_{-m}-\bbeta_{-m}^*\|_1$, we turn to bound $\|\nabla l(\bbeta^*_{-m},\bgamma^*_m;\hat{\vf}_m)\|_\infty$. 
  We estimate $\|\nabla_{\bgamma_m} l(\bbeta^*_{-m},\bgamma^*_m;\hat{\vf}_m)\|_\infty$ and $\|\nabla_{\bbeta_{-m}} l(\bbeta^*_{-m},\bgamma^*_m;\hat{\vf}_m)\|_\infty$ separately.
  For $\|\nabla_{\bgamma_m} l(\bbeta^*_{-m},\bgamma^*_m;\hat{\vf}_m)\|_\infty$, in view of Lemma \ref{lemm1}, 
    $$
    \max_{i\in[n]}\|\hat{\vf}_{i,m}-\vf_{i,m}\|_\infty\le C\left[\sqrt{\frac{\log(n)}{p_m}}+\sqrt{\frac{\log (p_m)\log (n)}{n}}\right] 
    $$
    holds with probability tending to one for some positive constant $C>0$. Then similarly to the proof of $\|I_2^{(1)}\|_\infty=o_p(n^{-1/2})$ in Theorem \ref{theorem1},  by the Bernstein inequality and the union bound, we have
    \begin{align} \label{beta_est1}
        \|\nabla_{\bgamma_m} l(\bbeta^*_{-m},\bgamma^*_m;\hat{\vf}_m)\|_\infty=O_p\left\{\sqrt{\frac{\log(n)}{p_m}}+\sqrt{\frac{\log (p_m)\log (n)}{n}}\right\}. 
    \end{align}
    For $\|\nabla_{\bbeta_{-m}} l(\bbeta^*_{-m},\bgamma^*_m;\hat{\vf}_m)\|_\infty$, it follows from Lemma 3.3 of \cite{lasso2013} that 
    \begin{align} \label{beta_est2}
        \|\nabla_{\bbeta_{-m}} l(\bbeta^*_{-m},\bgamma^*_m;{\vf}_m)\|_\infty=O_p\left\{\kappa_{n,p}\sqrt{\frac{\log (p-p_m)}{n}}\right\},
    \end{align}
    where $\kappa_{n,p}=\sqrt{\log\big[n(p-p_m)\big]}$. On the other hand, similarly to the proof of $|I_{1,k}|=o_p(n^{-1/2})$ in Theorem \ref{theorem1}, we have
    \begin{align} \label{beta_est3}
        \|\nabla_{\bbeta_{-m}} l(\bbeta^*_{-m},\bgamma^*_m;\hat{\vf}_m)-\nabla_{\bbeta_{-m}} l(\bbeta^*_{-m},\bgamma^*_m;{\vf}_m)\|_\infty=O_p\left\{\sqrt{\frac{\log(n)}{p_m}}+\sqrt{\frac{\log (p_m)\log (n)}{n}}\right\}.
    \end{align}
    Combining (\ref{beta_est1}), (\ref{beta_est2}) and (\ref{beta_est3}), we have 
    $$
    \|\nabla l(\bbeta^*_{-m},\bgamma^*_m;\hat{\vf}_m)\|_\infty=O_p\left\{\sqrt{\frac{\log(n)}{p_m}}+\sqrt{\frac{\log (p_m)\log (n)}{n}}+\kappa_{n,p}\sqrt{\frac{\log (p-p_m)}{n}}\right\}.
    $$
    Noting that $\lambda_1 \asymp \sqrt{{\log(n)}/{p_m}}+\sqrt{{\log (p_m)\log (n)}/{n}}+\kappa_{n,p}\sqrt{\log (p-p_m)/n}$ and $\xi$ is a some positive constant, we complete the proof of the first part of Lemma~\ref{lemm2}.

We now derive a bound for $\big\|\hat{\bw}_k-\bw_k^*\big\|_1$. For the $k$-th column of $\bW$, we solve
    \begin{align} \label{S4}
        &\hat{\bw}_k=\operatorname{argmin}\left\|\bw_k\right\|_1, \notag  \\
        \text{subject~~to}~~&\left\| \nabla^2_{\bbeta_{-m},\gamma_{m_k}} {l}(\hat\bbeta_{-m},\hat\bgamma_{m};\hat{\vf}_m)- \left(\nabla^2_{\bbeta_{-m},\bbeta_{-m}} {l}(\hat\bbeta_{-m},\hat\bgamma_{m};\hat{\vf}_m)\right)\bw_k \right\|_{\infty} \leq \lambda_2. 
    \end{align}
    Let $S_k=\text{supp}(\bw_k^*) $, where $\bw_k^*$ is the $k$-th column of $\bW^*$. By the definition of $\hat{\bw}_k$ in (\ref{S4}), we have $\|\bw^*_{S_k}\|_1\ge\|\hat\bw_{S_k}\|_1+\|\hat\bw_{S_k^c}\|_1$. By the triangle inequality, we obtain 
    $$
    \begin{aligned}
        \left\|\bw^*_{S_k}\right\|_1\ge &\left\|\hat\bw_{S_k}\right\|_1+\left\|\hat\bw_{S_k^c}\right\|_1 \\
        \ge &\left\|\bw^*_{S_k}\right\|_1-\left\|\hat{\bw}_{S_k}-\bw^*_{S_k}\right\|_1+\left\|\hat\bw_{S_k^c}\right\|_1,
    \end{aligned}
    $$
    which implies 
    \begin{align} \label{Sw1}
        \left\|\hat{\bw}_{S_k}-\bw^*_{S_k}\right\|_1\ge\left\|\hat\bw_{S_k^c}\right\|_1.
    \end{align} 
    Let $\hat\bDelta_k=\hat\bw_k-\bw^*_k$. Note $\bw^*_{S_k^c}=\mathbf 0$. Then it follows from (\ref{Sw1}) that 
    \begin{align} \label{Sw2}
        \left\|\hat\bDelta_{S_k}\right\|_1\ge\left\|\hat\bDelta_{S_k^c}\right\|_1.
    \end{align}
    Denote $\bH_x=\nabla^2_{\bbeta_{-m},\bbeta_{-m}} {l}(\hat\bbeta_{-m},\hat\bgamma_{m};\hat{\vf}_m)$ and $\bH_{xf}=\nabla^2_{\bbeta_{-m},\gamma_{m_k}} {l}(\hat\bbeta_{-m},\hat\bgamma_{m};\hat{\vf}_m)$. It follows from Lemma~\ref{lemma3} that 
    $$
    \left\|\bH_{xf}-\bH_{x}\bw_k^*\right\|_\infty=O_p(C^\prime_{n,p_m,p-p_m}).
    $$
    Together with (\ref{S4}), we have
    \begin{align}\label{hao1}
        \left\|\bH_x\hat\bDelta_k\right\|_\infty\le &\left\|\bH_{xf}-\bH_{x}\hat{\bw}_k\right\|_\infty+\left\|\bH_{xf}-\bH_{x}\bw_k^*\right\|_\infty 
        =O_p(C^\prime_{n,p_m,p-p_m}).
    \end{align}
Then, from (\ref{Sw2}), we obtain
    \begin{align} \label{Sw3}
        \left\|\hat{\bDelta}_k\right\|_1=\left\|\hat{\bDelta}_{S_k}\right\|_1+\left\|\hat{\bDelta}_{S_k^c}\right\|_1\le 2\left\|\hat{\bDelta}_{S_k}\right\|_1\le 2\sqrt{s_k^*}\left\|\hat{\bDelta}_{S_k}\right\|_2\le 2\sqrt{s_k^*}\left\|\hat{\bDelta}_k\right\|_2.
    \end{align}
    Thus, combining (\ref{hao1}) and (\ref{Sw3}), we get
    \begin{align} \label{S5}
    \hat{\bDelta}_k^\top\bH_x\hat{\bDelta}_k&\le\left\|\hat{\bDelta}_k\right\|_1\left\|\bH_x\hat{\bDelta}_k
    \right\|_\infty \notag \\
    &=O_p\left(\left\|\hat{\bDelta}_k\right\|_1C^\prime_{n,p_m,p-p_m}\right) 
    =O_p\left(\left\|\hat{\bDelta}_k\right\|_2\sqrt{s_k^*}C^\prime_{n,p_m,p-p_m}\right). 
    \end{align}
    It follows from Proposition 1 of \cite{Raskutti} that the restricted eigenvalue condition holds for $\bH_x$ with probability tending to one, i.e., $\hat{\bDelta}_k^\top\bH_x\hat{\bDelta}_k\ge\nu\|\hat{\bDelta}_k\|_2^2$ for some $\nu>0$ and all $\hat{\bDelta}_k$ that satisfy $\|\hat\bDelta_{S_k}\|_1\ge\|\hat\bDelta_{S_k^c}\|_1$. Together with (\ref{S5}), we have 
    $$
    \nu\left\|\hat{\bDelta}_k\right\|_2^2\le\hat{\bDelta}_k^\top\bH_x\hat{\bDelta}_k=O_p\left(\left\|\hat{\bDelta}_k\right\|_2\sqrt{s_k^*}C^\prime_{n,p_m,p-p_m}\right),
    $$
    which implies
    $$
    \left\|\hat{\bDelta}_k\right\|_2=O_p\left(\sqrt{s_k^*}C^\prime_{n,p_m,p-p_m}\right).
    $$
    Hence by (\ref{Sw3}),
    $$
    \left\|\hat{\bDelta}_k\right\|_1\le 2\sqrt{s_k^*}\left\|\hat{\bDelta}_k\right\|_2=O_p\left(s_k^*C^\prime_{n,p_m,p-p_m}\right)=O_p(s_k^*\lambda_2).
    $$
    This completes the proof of Lemma~\ref{lemm2}.

\section{Additional lemmas}

\setcounter{lemma}{0}

\renewcommand{\thelemma}{S\arabic{lemma}}

\begin{lemma}\label{lemm1}
        Suppose that Assumptions \ref{asym:Iden}-\ref{asym:lod} hold. If the random variable $\|\bx_m\|_2$ and $\|\bB_m^\top\bu_m\|_2$ are sub-Gaussian, then
        $$
        \max_{i\in[n]}\left\|\hat{\vf}_{i,m}-\vf_{i,m}\right\|_2=O_p\left\{\sqrt{\frac{\log (n)}{p_m}}+\sqrt{\frac{\log (p_m)\log (n)}{n}}\right\}.
        $$
        In addition, if $\|\vf_m\|_2$ is sub-Gaussian, then
        $$
        \max_{i\in[n]}\left\|\hat{\bu}_{i,m}-\bu_{i,m}\right\|_\infty=O_p\left\{\sqrt{\frac{\log (n)}{p_m}}+\sqrt{\frac{\log (p_m)\log (n)}{n}}\right\}.
        $$
        Furthermore, if $\|\bx_m\|_\infty$ and $\|\vf_m\|_\infty$ are bounded and $\|\bB_m^\top\bu_m\|_\infty\le C$ for some positive constant $C$, then
        $$
        \begin{aligned}
            &\max_{i\in[n]}\left\|\hat{\vf}_{i,m}-\vf_{i,m}\right\|_2=O_p\left(\sqrt{\frac{\log (p_m)}{n}}+\sqrt{\frac{1}{p_m}}\right), \\
            &\max_{i\in[n]}\left\|\hat{\bu}_{i,m}-\bu_{i,m}\right\|_\infty=O_p\left(\sqrt{\frac{\log (p_m)}{n}}+\sqrt{\frac{1}{p_m}}\right).
        \end{aligned}
        $$
\end{lemma}

\noindent{\it Proof.} This lemma follows directly from Lemma 3.1 of \cite{fan2022}.

\begin{lemma}\label{lemma3}
    Suppose that the assumptions of Theorem~\ref{theorem1} hold. Then
    $$
    \left\| \nabla^2_{\bbeta_{-m},\gamma_{m_k}} {l}(\hat\bbeta_{-m},\hat\bgamma_{m};\hat{\vf}_m)- \nabla^2_{\bbeta_{-m},\bbeta_{-m}} {l}(\hat\bbeta_{-m},\hat\bgamma_{m};\hat{\vf}_m)  {\bw^*_k}\right\|_{\infty} = O_p(C^\prime_{n,p_m,p-p_m}),
    $$
    where $\gamma_{m_k}$ is the $k$-th element of $\bgamma_m$.
\end{lemma}
    
    \noindent{\it Proof.} Recall  
    $$
    l(\bbeta_{-m},\bgamma_{m};{\vf}_m)=-\frac{1}{n}\sum_{i=1}^n\int_0^\tau(\vf_{i,m}^\top\bgamma_m+\bx_{j,-m}^\top\bbeta_{-m})dN_i(t)+\frac{1}{n}\sum_{i=1}^n\int_0^\tau\log\bPhi_0(t,\btheta_m,\vf_m)dN_i(t).
    $$
    Similarly to the proof of $\|I_2^{(1)}\|_\infty=o_p(n^{-1/2})$ in Theorem \ref{theorem1},  by the Bernstein inequality and the union bound, we have
    \begin{align} \label{lemmaS2.1}
        \left\| \nabla^2_{\bbeta_{-m},\gamma_{m_k}} l(\hat\bbeta_{-m},\hat\bgamma_{m};\vf_m)- \nabla^2_{\bbeta_{-m},\bbeta_{-m}} l(\hat\bbeta_{-m},\hat\bgamma_{m};\vf_m)\bw^*_k \right\|_{\infty} = O_p\left(\sqrt{\frac{\log (p-p_m)}{n}}\right).
    \end{align}
   In addition, we have
    \begin{align} \label{lemmaS2.2}
        &\left\| \nabla^2_{\bbeta_{-m},\gamma_{m_k}} [{l}(\hat\bbeta_{-m},\hat\bgamma_{m};\hat{\vf}_m)-{l}(\hat\bbeta_{-m},\hat\bgamma_{m};{\vf}_m)]- \nabla^2_{\bbeta_{-m},\bbeta_{-m}}[{l}(\hat\bbeta_{-m},\hat\bgamma_{m};\hat{\vf}_m)-{l}(\hat\bbeta_{-m},\hat\bgamma_{m};{\vf}_m)] \bw^*_k \right\|_{\infty} \notag \\
        &\le\max_{i\in[n]}\left|\hat f_{i,m_k}- f_{i,m_k}\right| O_p\left(\sqrt{\frac{\log (p-p_m)}{n}}\right)  \notag \\
        &\le\max_{i\in[n]}\left\|\hat\vf_{i,m}-\vf_{i,m}\right\|_2 O_p\left(\sqrt{\frac{\log (p-p_m)}{n}}\right)  \notag \\
        &=O_p\left\{\sqrt{\frac{\log (n)}{p_m}}+\sqrt{\frac{\log (p_m)\log (n)}{n}}\right\}O_p\left(\sqrt{\frac{\log (p-p_m)}{n}}\right),
    \end{align}
    where the last equality follows from Lemma~\ref{lemm1}. Combining (\ref{lemmaS2.1}) and (\ref{lemmaS2.2}), we complete the proof.

\bibliography{ref}  

\end{document}
